# Supplementary material for: Predictions of damages from Atlantic tropical cyclones: a hierarchical Bayesian study on extremes
Source: arXiv:2208.07899 source file (2025-06-11)

# A Supplementary: Model Details, and Additional Data Analysis

## A.1 Bayesian Model For Seasonal Analysis: Details

Recall that the cyclones are in two groups, low and high intensity, and we use the generic notation  $C$  for a group. Let occurrence frequency of group  $C$  in year  $i$  be represented by  $N_{C,i}$ , and let the frequency of damage-causing cyclones in group  $C$  in year  $i$  be represented by  $L_{C,i}$ . Finally, let damages in year  $i$  be represented as  $D_{C,i}$ . Let the corresponding vector collections of all years for these variables be  $\mathbf{N}_C$ ,  $\mathbf{L}_C$ , and  $\mathbf{D}_C$ . For a given year,  $i$ , define annual covariates as  $X_i$ .

The distribution of annual low intensity cyclone frequencies is modeled as a negative binomial distribution. In (12), we parameterize the negative binomial density for observation  $i$  with  $p_i$  and  $r$ . The latter is the (over)dispersion parameter, which in the Poisson distribution equals 1 (no overdispersion). The former is referred to as the success parameter, and for observation  $i$  is defined as  $p_i = r/(r + \lambda_i)$ , where  $\log \lambda_i = \sum_j \beta_j X_{ij}$ .

Frequency of damage-inflicting tropical cyclones,  $\mathbf{L}_1$ , is modeled using a binomial distribution with parameter  $\theta_1$  in (2) based on the elements in the vector of annual frequencies,  $\mathbf{N}_1$ . Finally, damages,  $\mathbf{D}_1$ , are modeled in (3) using a mixture distribution with a mass at 0 and nonzero damage modeled by a lognormal distribution with parameter  $(\mu_1, \sigma_1)$ .

Priors are specified independently and employ normal distributions for  $\beta_1$ , and  $\mu_1$  as in (15) and (17), respectively. The distribution of  $\theta_1$  is specified in (16) using a Beta distribution and  $\sigma_1$  in (18) using an inverse transformation to a Gamma distribution. In addition, we use a uniform prior that puts an upper bound of 70 for  $r$ , as in (19). This is not restrictive as the negative binomial tends to the Poisson as  $r \rightarrow \infty$ .

The hierarchical specification for the high intensity cyclones is similar to that of low intensity save for the cyclone occurrence distribution. Cyclone occurrence in (21) utilizes a Poisson distribution with mean parameter,  $\gamma(\mathbf{X}) = \mathbf{X}\beta_2$ . As in the low intensity case, the frequency of damage-inflicting cyclones,  $\mathbf{L}_2$ , is modeled using a binomial distribution with parameter  $\theta_2$  in (22) based on the vector of annual frequencies,  $\mathbf{N}_2$ . Finally, damages,  $\mathbf{D}_2$ , are modeled in (23) using a mixture distribution with a mass at 0 and nonzero damage modeled by a lognormal distribution with parameter  $(\mu_2, \sigma_2)$ . Priors are specified independently and employ normal distributions for  $\beta_2$  and  $\mu_2$  as in (24) and (26), respectively. The distribution of  $\beta_2$  is specified with independent components. Similar to the low intensity case,  $\theta_2$  is specified using a Beta distribution in (25), and  $\sigma_2$  is specified in (27) using an inverse transformation to a Gamma distribution.

Below, we specify the precise model that we used in this paper. We use the notations  $\mathbf{0}_{q_1}$  for a vector of 0s of length  $q$  and  $I_q$  for an identity matrix of size  $q \times q$  where  $q$  depends on the number of covariates in the model being fit.

### Low Intensity Cyclone Fully Bayesian Specification:

$$[N_{1,i}|X_i, r, p_i, \beta_1] \sim \text{NegBinom}(r, p_i) \quad (12)$$

$$p_i = \frac{r}{r + \lambda(x_i)}$$

$$\log(\lambda(x_i)) = x_i \beta_1; \beta_1 \in \mathbb{R}^{q_1}$$

$$[L_{1,i}|N_{1,i}, X_i, \phi, \beta_1, \theta_1] \sim \text{Binomial}(n_{1,i}, \theta_1) \quad (13)$$

$$[D_{1,i}|L_{1,i}, N_{1,i}, X_i, \phi, \beta_1, \theta_1, \mu_1, \sigma_1] \sim (1 - (1 - \theta_1)^{n_{i1}}) * \text{Lognormal}(\mu_1, \sigma_1) + (1 - \theta_1)^{n_{i1}} * 0 \quad (14)$$

$$[\beta_1] \sim \mathcal{N}(\mathbf{0}_{q_1}, 10^5 I_{q_1}) \quad (15)$$

$$[\theta_1] \sim \text{Beta}(1, 1) \quad (16)$$

$$[\mu_1] \sim \mathcal{N}(0, 10^5) \quad (17)$$

$$\left[ \frac{1}{\sigma_1^2} \right] \sim \text{Gamma}(1, 1) \quad (18)$$

$$[r] \sim \text{Unif}(0, 70) \quad (19)$$

### High Intensity Cyclone Fully Bayesian Specification:

$$[N_{2,i}|X_i, \beta_2] \sim \text{Poisson}(\lambda(x_i)) \quad (20)$$

$$\log(\lambda(x_i)) = x_i \beta_2; \beta_2 \in \mathbb{R}^{q_2} \quad (21)$$

$$[L_{2,i}|N_{2,i}, X_i, \beta_2, \theta_2] \sim \text{Binomial}(n_{2,i}, \theta_2) \quad (22)$$

$$[D_{2,i}|L_{2,i}, N_{2,i}, X_i, \beta_2, \theta_2, \mu_2, \sigma_2] \sim (1 - (1 - \theta_2)^{n_{i2}}) * \text{Lognormal}(\mu_2, \sigma_2) + (1 - \theta_2)^{n_{i2}} * 0 \quad (23)$$

$$[\beta_2] \sim \mathcal{N}(\mathbf{0}_{q_2}, 10^5 I_{q_2}) \quad (24)$$

$$[\theta_2] \sim \text{Beta}(1, 1) \quad (25)$$

$$[\mu_2] \sim \mathcal{N}(0, 10^5) \quad (26)$$

$$\left[ \frac{1}{\sigma_2^2} \right] \sim \text{Gamma}(1, 1) \quad (27)$$

## A.2 Additional Analysis: Empirical Bayesian Modeling Of Seasonal Data

To corroborate the full hierarchical Bayesian model presented in Section 5, we carried out multiple studies. One is an empirical Bayesian study, where we used the maximum likelihood estimators to inform the prior. The technical details are given below. As can be seen from Tables 3 and 4, the results from empirical Bayes are very close to those obtained using the hierarchical Bayesian model.

**Low Intensity Cyclone Bayesian Specification (EB):**

$$[N_{1,i}|X_i, r, p_i, \beta_1] \sim \text{NegBinom}(r, p_i) \quad (28)$$

$$p_i = \frac{r}{r + \lambda(x_i)}$$

$$\log(\lambda(x_i)) = x_i \beta_1; \beta_1 \in \mathbb{R}^{q_1}$$

$$[L_{1,i}|N_{1,i}, X_i, \phi, \beta_1, \theta_1] \sim \text{Binomial}(n_{1,i}, \theta_1) \quad (29)$$

$$[D_{1,i}|L_{1,i}, N_{1,i}, X_i, \phi, \beta_1, \theta_1, \mu_1, \sigma_1] \sim (1 - (1 - \theta_1)^{n_{i1}}) * \text{Lognormal}(\mu_1, \sigma_1) + (1 - \theta_1)^{n_{i1}} * 0 \quad (30)$$

$$[\beta_1] \sim \mathcal{N}((\hat{\beta}_{11}, \dots, \hat{\beta}_{1q_1}), 10^4 I_{q_1}) \quad (31)$$

$$[\log(\phi)] \sim \mathcal{N}(\log(\hat{\phi}), 1) \quad (32)$$

$$[\theta_1] \sim \text{Beta}(\alpha(\hat{p}_1), \beta(\hat{p}_1)) \quad (33)$$

$$[\mu_1] \sim \mathcal{N}(\bar{x}_1, 10^4) \quad (34)$$

$$[r] \sim \text{Unif}(0, 70) \quad (35)$$

$$\left[ \frac{1}{\sigma_1^2} \right] \sim \text{Gamma}(v_{11}(\hat{s}_1), v_{12}(\hat{s}_1)) \quad (36)$$

**High Intensity Cyclone Bayesian Specification (EB):**

$$[N_{2,i}|X_i, \beta_2] \sim \text{Poisson}(\lambda(x_i)) \quad (37)$$

$$\log(\lambda(x_i)) = x_i \beta_2; \beta_2 \in \mathbb{R}^{q_2}$$

$$[L_{2,i}|N_{2,i}, X_i, \beta_2, \theta_2] \sim \text{Binomial}(n_{2,i}, \theta_2) \quad (38)$$

$$[D_{2,i}|L_{2,i}, N_{2,i}, X_i, \beta_2, \theta_2, \mu_2, \sigma_2] \sim (1 - (1 - \theta_2)^{n_{i2}}) * \text{Lognormal}(\mu_2, \sigma_2) + (1 - \theta_2)^{n_{i2}} * 0 \quad (39)$$

$$[\beta_2] \sim \mathcal{N}([\hat{\beta}_{21}, \dots, \hat{\beta}_{2q_2}]^T, 10^4 I_{q_2}) \quad (40)$$

$$[\theta_2] \sim \text{Beta}(\alpha(\hat{p}_2), \beta(\hat{p}_2)) \quad (41)$$

$$[\mu_2] \sim \mathcal{N}(\bar{x}_2, 10^4) \quad (42)$$

$$\left[ \frac{1}{\sigma_2^2} \right] \sim \text{Gamma}(v_{21}(\hat{s}_2), v_{22}(\hat{s}_2)) \quad (43)$$

### A.3 Additional Analysis: Data Clone Computations On Seasonal Data

In addition to the hierarchical Bayes and empirical Bayes computations, we also used `dclone`<sup>88</sup> method to analyze the data, and provide further support and justification about the robustness of our findings.

Data cloning was implemented using 1, 2, and 5 clones. We report the estimates of the the 5 clone chain. Each run consisted of running 3 chains of length 100,000 with adaptation on the first 100 iterations. The Markov Chain Monte Carlo (MCMC) procedure with Gibbs sampling was also implemented using 3 chains, each with 100,000 iterations. The first 100 iterations of each chain were discarded.

We report some comparison results across different statistical methodologies in Tables 3 and 4. Here, we either used all the covariates, or used a select few depending on a statistical model selection criterion (in these cases, both Akaike and Bayesian model selection suggested the same model, where a few covariates are dropped). We compare the empirical Bayesian approach with the full hierarchical Bayesian approach for both these choices. Model fitting was done either by MCMC, or by adapting the non-Bayesian data cloning approach. The tables report the posterior mean and standard deviation for the different parameter values, for these various combinations. Both tables demonstrate that there is little difference between the results from different techniques, and that we have excellent robustness against a choice of statistical methodology. Additional robustness studies were also conducted. We have used the hierarchical bayesian approach with all covariates as the main approach for the results reported in the paper.

## A.4 Seasonal Prediction Details

We utilize the Bayesian specification to get an estimate of the posterior predictive distribution. Let the distributional specification of the data  $\mathbf{Y} = [\mathbf{N}, \mathbf{L}, \mathbf{D}]$  given parameters  $\gamma = [\beta, \theta, \mu, \sigma, \phi]$  be  $p(y|\gamma)$ . Also, let the posterior distribution of  $\gamma$  given the data  $\mathbf{Y}$  and the hyperparameter  $\alpha$  be  $p(\gamma|y, \alpha)$ . Then, the posterior predictive distribution for a new observation,  $\tilde{\mathbf{Y}}$  is

$$p(\tilde{y}|y, \alpha) = \int p(\tilde{y}|\gamma)p(\gamma|y, \alpha)d\gamma \quad (44)$$

This is obtained computationally as follows:

1. Let  $\{\hat{\gamma}_i; i = 1, \dots, T\}$  be the MCMC set of posterior samples.
2. Using each of these posterior estimates, we sample a new  $y$  ( $N, L, D$ ) given  $\hat{\gamma}_i$  using the covariates for test data. We call this new  $y$  as  $y_{\text{pred}}^{(i)}$ .
3. Plot a histogram (density) using all the predicted  $y$ 's, i.e.,  $\{y_{\text{pred}}^{(i)}; i = 1, \dots, T\}$ .

Since the above steps involve massive computations, we also explored two simpler approaches, outlined below:

- **Empirical Bayesian prediction:**

1. Obtain the posterior sample mean from the hierarchical Bayesian model fit in Section 5, call them  $\hat{\gamma}_{HB}$ .
2. Sample  $10^5$  times from model specification  $p(\tilde{y}|\hat{\gamma}_{HB})$  for each of the response variables, i.e., frequency of cyclones, frequency of damage-inflicting cyclones and value of damages. This provides a single realization of the posterior predictive distribution.

- **Fast computation Bayesian prediction:**

1. Let  $\{\hat{\gamma}_i; i = 1, \dots, T\}$  be the MCMC set of posterior samples. Note,  $T$  is the number of posterior samples obtained in the MCMC output.
2. Using each of these posterior estimates, we sample  $y$  ( $N, L, D$ ),  $S = 1000$  times using the covariates for test data. We call this new  $y$  as  $y_{\text{pred}_j}^{(i)}$ .
- 3a. Now estimate the density  $p(\tilde{y}|\hat{\gamma}_i)$  using a kernel density estimate:

$$\hat{p}(\tilde{y}|\hat{\gamma}_i) = \frac{1}{Sh} \sum_{j=1}^S K\left(\frac{\tilde{y} - y_{\text{pred}_j}^{(i)}}{h}\right)$$

- 3b. The predictive posterior distribution can then be estimated as:

$$\hat{p}(\tilde{y}|y, \alpha) = \frac{\sum_{i=1}^T \hat{p}(\tilde{y}|\hat{\gamma}_i)}{T}$$

4. Sample from the predictive posterior distribution  $\hat{p}(\tilde{y}|y, \alpha)$ .

Predictive inference results for the above two methods are given in Section B, along with the fully hierarchical Bayesian prediction model given in Section 2. It can be seen that the results look very similar across the three methods of predictive posterior inference.

## B Appendix: Interpretation Of Posterior Predictive Densities (Seasonal Analysis)

We present a detailed discussion, and additional figures, for the Bayesian predictive analysis.

We discuss the results in detail for 2016-2019 below, to illustrate how the probability density or mass functions depicted in these figures reflect the data. In each analysis, we use the hierarchical Bayesian model, described in Section 2, the empirical Bayesian prediction and the fast computation Bayesian prediction, both described in Section A.4.

### B.1 2016 Posterior Predictive Bayesian Analysis

The results are presented in Figure 5 for low intensity cyclones and in Figure 6 for high intensity cyclones. The results for 2016 indicate the model matches well with the data. The three posterior predictive methods provide similar output except that the second method has slightly more variability and provides a smoother density curve because of the averaging. As seen in Figure 5 (three figures in first (left) panel/column), the actual number of cyclones was well within the predicted distribution for the low intensity category and had at least 30% of the probability higher than the observed value. Similarly, in Figure 6 (first column), high intensity cyclone occurrence, although falling at the start of the right tail end, was within the limits of the predictive distribution.

For low intensity tropical cyclones, the predictive distribution in Figure 5(three figures in the second (middle) column) indicated that a given cyclone would inflict damages in 2016, was given approximately a 31-32% chance in each of the three versions of posterior predictive distributions. The corresponding figures for high intensity damage-inflicting cyclones in Figure 6(second column) are around 31-32%. There were \$550 million in low intensity damages, thus, Figure 5(three figures in the third (right) column) reflect the actual amount of damage for 2016 falls well within the predicted distribution for the low intensity category with non-zero damages. There were a \$ 1 billion in high intensity damages in 2016. The high intensity damages in Figure 6(third column) indicate that the true value of damage falls well within the posterior predictive range for the non-zero values. Although, there is a greater chance of no (\$0) damages (about 55%) and the log of damage incurred in 2016 had about an 8% chance of occurrence.

## B.2 2017 Posterior Predictive Bayesian Analysis

Similar to 2016, results for 2017 indicate the model matches well with the observations. Again, the two posterior predictive methods provide similar output with the second method showing more variability and a smoother density curve.

As seen in Figure 7(three figures in first (left) column), the actual number of cyclones was well within the predicted distribution for the low intensity category and had at least 30% of the probability higher than the observed value. Similarly, in Figure 8(first column), high intensity cyclone occurrence, although falling at the start of the right tail end, was within the limits of the predictive distribution.

From Figure 7(three figures in the second (middle) column) indicated that in 2017, a low intensity cyclone has the probability of about 33-34% for causing damages in each of the three versions of posterior predictive distributions. Observing two high intensity damage-inflicting cyclones as in 2017 had approximately a 23-24% chance in Figure 8(middle column). There were \$225 million in low intensity damages, thus, Figure 7(three figures in the third (right) column) reflect the chance of the corresponding damage appropriately and the log of the actual amount of damage for 2017 falls well within the predicted distribution for the low intensity category with non-zero damages. The high intensity damages in Figure 8(third column) indicate the log of damage incurred in 2017 (\$175 billion) although slightly in the right end of the distribution with about an 2-3% chance of occurrence.

## B.3 2018 Posterior Predictive Bayesian Analysis

Similar to the previous two years results for 2018 indicate the model matches well with the observations. Again, the three posterior predictive methods provide similar output with the second method showing a smoother density curve for damages because of the averaging. A major difference with the previous two years here is that the true damage value for 2018 (marked in red) is \$0.

The results for 2018 indicate the model matches well with the data. As seen in Figure 9(three figures in first (left) column), the actual number of cyclones was well within the predicted distributions. Similarly, in Figure 10(first column), high intensity cyclone occurrence was also within the limits of the predictive distribution. The observed value of 2 cyclones accounted for nearly 24% of the samples.

For low intensity tropical cyclones, the predictive distribution in Figure 9(three figures in second column) indicated that observing no damage-inflicting cyclone, as in 2018, was given approximately a 22-23% chance in each of the three versions of posterior predictive distributions. Similarly, observing no high intensity damage-inflicting cyclone as in 2018 had the probability in Figure 10(middle column) at around 36-37%. There were \$0 in low intensity as well as high intensity damages, thus, Figure 9(three figures in last (right) column), and Figure 11 (third column) reflect the chance of no damages appropriately and the actual amount of damage for 2018 falls well within the predicted distribution with about a 23% chance for the low intensity category and 37% change for the high intensity category, respectively, for zero damages.

## B.4 2019 Posterior Predictive Bayesian Analysis

Similar to the previous three years results for 2019 indicate the model matches well with the observations. Again, the three posterior predictive methods provide similar output with the second method showing a smoother density curve for damages because of the averaging. Note that the true damage value for 2019 (marked in red) is also \$0.

The results for 2019 indicate the model matches well with the data, as seen in Figure 11(three figures in first (left) column) and in Figure 12(left column).

For low intensity tropical cyclones, the predictive distribution in Figure 11(three figures in second (middle) column) indicated that observing no damage-inflicting cyclone, as in 2019, was given approximately a 22-23% chance in each of the three versions of posterior predictive distributions. Similarly, observing zero high intensity damage-inflicting cyclone had the probability in Figure 12(middle column) at around 36-37%. There were \$0 in low intensity as well as high intensity damages, thus, Figure 11(three figures in last (right) column), and Figure 12 (last column) reflect the chance of no damages appropriately and the actual amount of damage for 2018 falls well within the predicted distribution with about a 22% chance for the low intensity category and 38% change for the high intensity category, respectively, for zero damages.

## C Appendix: Additional Analysis Of Individual Cyclones Data

### C.1 Individuation Cyclones: Trivariate Extreme Value Model

Here, we model  $\mathbf{Y} = [\mathbf{maxWS}, \mathbf{minCP}, \mathbf{Damage}]$  using a trivariate extreme values distribution (GEV) model. Let  $X_1$  denote the logarithm of maxWS,  $X_2$  denote logarithm of damages and  $Z_1$  denote the logarithm of minCP. We also add non-stationarity in the location parameters to fully utilize all information, including the average latitudes, namely,  $Z_2$ . We consider the following hierarchy in modeling the location parameters,

$$\begin{aligned}\mu_{z_1}(Z_2) &= \alpha_0 + \alpha_1 Z_2 \\ \mu_{x_1}(Z_1, Z_2) &= \beta_0 + \beta_1 Z_1 + \beta_2 Z_2 \\ \mu_{x_2}(X_1, Z_1, Z_2) &= \gamma_0 + \gamma_1 X_1 + \gamma_2 Z_1 + \gamma_3 Z_2.\end{aligned}$$

The location and scale parameters have subscripts indicating the variable they represent. The joint distribution of a logistic dependence model<sup>89</sup> for three variables  $(Z_1, X_1, X_2)$  is given by,

$$G(z_1, x_1, x_2) = \exp(-(t(z_1)^{1/r} + t(x_1)^{1/r} + t(x_2)^{1/r})^r),$$

where  $r$  ( $0 < r \leq 1$ ) is the dependence parameter. We can differentiate this w.r.t.  $z_1, x_1, x_2$  to derive the density.

$$\begin{aligned}g(z_1, x_1, x_2) &= \frac{t(z_1)^{\xi_{z_1}+1}}{\sigma_{z_1}} \frac{t(x_1)^{\xi_{x_1}+1}}{\sigma_{x_1}} \frac{t(x_2)^{\xi_{x_2}+1}}{\sigma_{x_2}} t(z_1)^{\frac{1}{r}-1} t(x_1)^{\frac{1}{r}-1} t(x_2)^{\frac{1}{r}-1} \\ &\times \exp(-(t(z_1)^{1/r} + t(x_1)^{1/r} + t(x_2)^{1/r})^r) \\ &\times \left[ \frac{(1-r)(2-r)}{r} - \left( \frac{1-r}{r} \right) (t(z_1)^{1/r} + t(x_1)^{1/r} + t(x_2)^{1/r})^r \right. \\ &\quad \left. + (t(z_1)^{1/r} + t(x_1)^{1/r} + t(x_2)^{1/r})^{2r} \right] \\ &\times (t(z_1)^{1/r} + t(x_1)^{1/r} + t(x_2)^{1/r})^{r-3}.\end{aligned}$$



Then the log-likelihood is given by,

$$\begin{aligned}
& l(\theta|Z_1, X_2, X_1; Z_2) \\
&= \sum_{i=1}^n \left( (\xi_{z_1} + 1) \log(t(z_{1i})) - \log(\sigma_{z_1}) + (\xi_{x_1} + 1) \log(t(x_{1i})) - \log(\sigma_{x_1}) \right. \\
&\quad + (\xi_{x_2} + 1) \log(t(x_{2i})) - \log(\sigma_{x_2}) + \left( \frac{1}{r} - 1 \right) \log(t(z_{1i})) \\
&\quad + \left( \frac{1}{r} - 1 \right) \log(t(x_{1i})) + \left( \frac{1}{r} - 1 \right) \log(t(x_{2i})) \\
&\quad - (t(z_{1i})^{1/r} + t(x_{1i})^{1/r} + t(x_{2i})^{1/r})^r \\
&\quad + \log \left[ \frac{(1-r)(2-r)}{r} \right. \\
&\quad \left. - \left( \frac{1-r}{r} \right) (t(z_{1i})^{1/r} + t(x_{1i})^{1/r} + t(x_{2i})^{1/r})^r \right. \\
&\quad \left. + (t(z_{1i})^{1/r} + t(x_{1i})^{1/r} + t(x_{2i})^{1/r})^{2r} \right] \\
&\quad \left. + (r-3) \log(t(z_{1i})^{1/r} + t(x_{1i})^{1/r} + t(x_{2i})^{1/r}) \right)
\end{aligned}$$

**Priors:**

$$\begin{aligned}
& \alpha_0, \alpha_1, \beta_0, \beta_1, \beta_2 \stackrel{iid}{\sim} N(0, 10^2) \\
& \gamma_0, \gamma_1, \gamma_2, \gamma_3 \stackrel{iid}{\sim} N(0, 10^3) \\
& \sigma_{z_1}, \sigma_{x_1}, \sigma_{x_2} \stackrel{iid}{\sim} \text{IG}(\alpha = 1, \beta = 1) \\
& \xi_{z_1} \sim \text{Unif}(-1, 1) \\
& \xi_{x_1}, \xi_{x_2} \stackrel{iid}{\sim} \text{Unif}(-0.5, 0.5) \\
& r \sim \text{Unif}(-0.05, 1)
\end{aligned}$$

The priors have been chosen based on well-known information about GEV models and keeping in the mind the frequentist univariate model estimates. The standard regularity conditions for the likelihood of an GEV are satisfied for  $\xi < 0.5$ . In particular for the range of values  $-0.5 < \xi < 0.5$  are most often encountered in practice<sup>90</sup>. Hence, we model the shape parameters by a uniform prior between -0.5 and 0.5. Since, in our parameterization of the dependence parameter,  $r$ ,  $0 < r \leq 1$ , we model it using a Uniform distribution but with a lower bound of 0.05 to avoid computational overflow. Other priors are non-informative.

We have 16 unknown parameters in this model and the step-sizes for the Metropolis Hastings (MH) algorithm have been chosen such that the acceptance rate for the MH-algorithm is about 20%, which is the generally accepted as a good enough acceptance rate. Note that we also standardize  $X_1$  to fit in the third model (as a covariate) as is recommended while fitting GEV models.

The Metropolis Hastings algorithm is run for  $10^6$  MCMC steps and we present the posterior means and standard deviations for the parameters in Table 5. We notice that while the estimates for the location parameters are close for the frequentist and the Bayesian models, the shape and scale parameter estimates vary. The shape parameter for  $Z_1$  ( $\log(\text{minCP})$ ) is -0.586 in the frequentist model while it is -0.434 for the Bayesian trivariate GEV model, which is within the consistency range for the MLE of the shape parameter,  $\xi$ . The shape parameter estimate for  $X_1$  ( $\log(\text{maxWS})$ ) decreases from -0.352 in the frequentist univariate case to -0.487 in the Bayesian trivariate case, while the estimate for  $X_2$  ( $\log(\text{damages})$ ) increases from -0.327 in the frequentist univariate case to -0.184 in the Bayesian trivariate case. Interestingly, the estimate for dependence parameter  $r$  is 0.997 which is very close to 1 signifying independence between the three variables considered. We suspect that this is because the non-stationarity considered in location parameters already accounts for the dependence between the three variables. The results seem pretty stable on change on starting values and modifications to the prior specifications.

The results of Table 5 are very close to those of Table 1, where we obtained the results using the hierarchical Bayesian GEV model. Thus, the conclusions from the data are quite robust to the data science framework used for analysis.

## C.2 Individuation Cyclones: Hierarchical Model with Log-Normal Damage

Since it is possible that cyclone damages follow a heavy-tailed but not necessarily extreme valued distribution, we model it has a log-normal distribution in this section. The overall structure remains the same as Section 6. Note,  $Z_1$  represents  $\log(\text{minCP})$ ,  $Z_2$  is for standardized average latitude,  $X_1$  represents  $\log(\text{maxWS})$  and  $X_2$  is for damages. We consider the following model:

$$Z_1|Z_2 \sim \text{GEV}(\mu_{z_1}(Z_2), \sigma_{z_1}, \xi_{z_1}) \quad (45)$$

$$X_1|(Z_1, Z_2) \sim \text{GEV}(\mu_{x_1}(Z_1, Z_2), \sigma_{x_1}, \xi_{x_1}) \quad (46)$$

$$X_2|(X_1, Z_1, Z_2) \sim \text{Lognormal}(\mu_{x_2}(X_1, Z_1, Z_2), \sigma_{x_2}), \quad (47)$$

where the hierarchy essentially comes in the location parameters,

$$\begin{aligned} \mu_{z_1}(Z_2) &= \alpha_0 + \alpha_1 Z_2 \\ \mu_{x_1}(Z_1, Z_2) &= \beta_0 + \beta_1 Z_1 + \beta_2 Z_2 \\ \mu_{x_2}(X_1, Z_1, Z_2) &= \gamma_0 + \gamma_1 X_1 + \gamma_2 Z_1 + \gamma_3 Z_2. \end{aligned}$$

The joint density can then be written as,

$$\begin{aligned}
& f(Z_1, X_1, X_2|Z_2, \theta) \\
&= f(X_2|X_1, Z_1, Z_2)f(X_1|Z_1, Z_2)f(Z_1|Z_2) \\
&= \frac{1}{x_2\sigma_{x_2}\sqrt{2\pi}} \exp\left(-\frac{(\log(x_2) - \mu_{x_2}(x_1, z_1, z_2))^2}{2\sigma_{x_2}^2}\right) \\
&\quad \times \frac{1}{\sigma_{x_1}} (t(x_1))^{\xi_{x_1}+1} \exp(-t(x_1)) \\
&\quad \times \frac{1}{\sigma_{z_1}} (t(z_1))^{\xi_{z_1}+1} \exp(-t(z_1)),
\end{aligned}$$

where,

$$t(x) = \begin{cases} (1 + \xi(\frac{x-\mu}{\sigma}))^{-1/\xi} & \xi \neq 0 \\ \exp(-\frac{x-\mu}{\sigma}) & \xi = 0. \end{cases}$$

Then the log-likelihood can be given by,

$$\begin{aligned}
l(\theta|X_1, X_2, Z_1, Z_2) &= \sum_{i=1}^n \left[ -\log(x_{2i}\sigma_{x_2}\sqrt{2\pi}) - \frac{(\log(x_{2i}) - \mu_{x_2})^2}{2\sigma_{x_2}^2} \right. \\
&\quad - \log(\sigma_{x_{1i}}) + (\xi_{x_{1i}} + 1) \log(t(x_{1i})) - t(x_{1i}) \\
&\quad \left. - \log(\sigma_{z_{1i}}) + (\xi_{z_{1i}} + 1) \log(t(z_{1i})) - t(z_{1i}) \right].
\end{aligned}$$

**Priors:** The location parameter priors for both the GEV models (minCP and maxWS) and the log-normal model (damages) are non-informative with variances chosen to be drawn for Inverse-Gamma(1,1) to ensure proper coverage of the sample space leading to good acceptance rates.

$$\begin{aligned}
\alpha_0, \alpha_1 &\stackrel{iid}{\sim} N(0, 10^3) \\
\beta_0, \beta_1, \beta_2 &\stackrel{iid}{\sim} N(0, 10^2) \\
\gamma_0, \gamma_1, \gamma_2, \gamma_3 &\stackrel{iid}{\sim} N(0, 10^3) \\
\sigma_{z_1}, \sigma_{x_1}, \sigma_{x_2} &\stackrel{iid}{\sim} \text{IG}(\alpha = 1, \beta = 1) \\
\xi_{z_1} &\sim \text{Unif}(-1, 1) \\
\xi_{x_1} &\stackrel{iid}{\sim} \text{Unif}(-0.5, 0.5).
\end{aligned}$$

We use Metropolis-Hastings algorithm to sample from the posterior distribution. The chain is run for  $N = 10^6$  MCMC sample size and the step-sizes are chosen to achieve about 20% acceptance rate. The results from this model fitting is given in Table 6. The results of this are very close to those in Table 5 and Table 1, where we reported the results using the trivariate Bayesian GEV model and the hierarchical Bayesian GEV model respectively. Thus, the conclusions from the data are quite robust to the data science framework used for analysis.

Note that the frequentist estimates for the location parameters are similar to the posterior means for the location parameters. The shape and scale parameters differ, similar to how they differed in the trivariate GEV model of Section C.1 and Bayesian hierarchical GEV model in Section 6. In terms of significance of estimates, coefficient of average latitude ( $\alpha_1$ ) in modeling location parameter for minCP is statistically significant. Similarly, the effect of minCP ( $\beta_1$ ) and average latitude ( $\beta_2$ ) in modeling location parameter for maxWS seems to be significant. The standard errors for the coefficient estimates for damages are high, resulting in non-significant effect corresponding to maxWS, minCP and average latitude, on the location parameter of damages, with a highly significant intercept term. The scale parameter estimates are significant across models, and the first two models in the hierarchy have a negative estimate for the shape parameters signifying Reverse Weibull distributions for the marginals of each of  $\log(\text{minCP})$  and  $\log(\text{maxWS})$  respectively.

### C.3 Individual Cyclones: Additional Predictions

Similar to the analysis presented in Section 3, we now present the prediction results for the Atlantic tropical cyclones of 2016-17 using the statistical models described in Section C.1 (trivariate Bayesian GEV) and in Section C.2 (hierarchical Bayesian model with log-Normal distribution for damages).

We consider the predictions from these models for the years 2016 and 2017. The details are same as those given in Section 3. We note from Table 7 that all the true minimum central pressure values were always within the 95% credible interval for all five cyclones. Even the true maximum wind speed fell within the intervals for all the three models, except it missed the mark very closely for hurricane Nate in hierarchical Bayesian model with log-Normal for damages. More specifically, the 95% credible interval for Nate was (3.1304, 4.3807) and the true value was 4.3820, on the log-scale. For damages, none of the credible intervals for the three models (hierarchical GEV in Section 3, trivariate GEV in Section C.1 and hierarchical model with log-Normal loss in Section C.2) could capture the observed value for Harvey in the 95% interval. However the damages due to Harvey is within the range of the posterior for the hierarchical GEV method of Section 3.

Similarly, the true damage value for Irma only fell in the 95% credible interval when the hierarchical GEV model of in Section 3 was fit, but was missed in the other two methods. However, the truth was not too far away in the tails of the predictive distribution. Given that Harvey and Irma both are in the top-five most damage causing Atlantic cyclones, these results are not surprising. We present the  $\delta$ -values using the models described in Section C.1 and in Section C.2 in Tables 8 and 9 respectively. These values are not substantially different from those of Table 2.

## D Appendix: All Tables

Table 3: Comparison of different statistical methodologies for analyzing the low intensity tropical cyclones data. Here, *all* refers to the model where all the covariates were used, while *selected* refers to where a few selected covariates were used. These were selected using a model selection criterion on a model with all covariates. The abbreviation EB refers empirical Bayes approach, while HB refers to hierarchical Bayesian approach that we use in the paper. The MCMC and dclone are two different computational approaches, the latter is non-Bayesian, but may be used in conjunction with empirical or hierarchical Bayesian techniques as well. Each entry is an expected value, with standard deviation in brackets. Results show excellent robustness across statistical methodologies.

| Parameter                  | Method | All             |                 | Selected        |                 |
|----------------------------|--------|-----------------|-----------------|-----------------|-----------------|
|                            |        | EB              | HB              | EB              | HB              |
| $\beta_{11}$<br>(NAO)      | MCMC   | -0.068 (0.059)  | -0.068 (0.059)  | -0.060 (0.059)  | -0.060 (0.059)  |
|                            | dclone | -0.068 (0.026)  | -0.068 (0.026)  | -0.060 (0.026)  | -0.060 (0.026)  |
| $\beta_{12}$<br>(SOI)      | MCMC   | -0.016 (0.031)  | -0.016 (0.031)  | -               | -               |
|                            | dclone | -0.016 (0.014)  | -0.016 (0.014)  | -               | -               |
| $\beta_{13}$<br>(AMO)      | MCMC   | -0.429 (0.211)  | -0.429 (0.211)  | -0.456 (0.208)  | -0.456 (0.208)  |
|                            | dclone | -0.429(0.092)   | -0.429 (0.092)  | -0.456 (0.092)  | -0.456 (0.092)  |
| $\beta_{14}$<br>Nino-3.4   | MCMC   | -0.253 (0.103)  | -0.254 (0.102)  | -0.207 (0.075)  | -0.207 (0.075)  |
|                            | dclone | -0.253 (0.045)  | -0.253 (0.045)  | -0.207 (0.033)  | -0.207 (0.033)  |
| $\beta_{15}$<br>(SST)      | MCMC   | 0.098 (0.003)   | 0.098 (0.003)   | 0.100 (0.002)   | 0.100 (0.002)   |
|                            | dclone | 0.098 (0.001)   | 0.098 (0.001)   | 0.100 (0.001)   | 0.100 (0.001)   |
| $\beta_{16}$<br>(Sunspots) | MCMC   | 0.001 (0.001)   | 0.001 (0.001)   | -               | -               |
|                            | dclone | 0.001 (0.000)   | 0.001 (0.000)   | -               | -               |
| $r$                        | MCMC   | 36.087 (15.590) | 36.065 (15.540) | 36.730 (15.474) | 36.807 (15.512) |
|                            | dclone | 37.118(11.046)  | 37.133 (11.064) | 34.932 (10.447) | 34.934 (10.439) |
| $\theta_1$                 | MCMC   | 0.142 (0.011)   | 0.142 (0.011)   | 0.142 (0.011)   | 0.142 (0.011)   |
|                            | dclone | 0.142 (0.005)   | 0.142 (0.005)   | 0.142 (0.005)   | 0.142 (0.005)   |
| $\mu_1$                    | MCMC   | 18.297 (0.344)  | 18.296 (0.337)  | 18.295 (0.344)  | 18.296 (0.337)  |
|                            | dclone | 18.296 (0.149)  | 18.295 (0.149)  | 18.296 (0.149)  | 18.296 (0.149)  |
| $\sigma_1^2$               | MCMC   | 5.074 (1.155)   | 4.882 (1.091)   | 5.077(1.161)    | 4.884 (1.093)   |
|                            | dclone | 4.790 (0.467)   | 4.756 (0.461)   | 4.789 (0.466)   | 4.756 (0.463)   |

Table 4: Comparison of different statistical methodologies for analyzing the high intensity tropical cyclones data. Here, *all* refers to the model where all the covariates were used, while *selected* refers to where a few selected covariates were used. These were selected using a model selection criterion on a model with all covariates. The abbreviation EB refers empirical Bayes approach, while HB refers to hierarchical Bayesian approach that we use in the paper. The MCMC and dclone are two different computational approaches, the latter is non-Bayesian, but may be used in conjunction with empirical or hierarchical Bayesian techniques as well. Each entry is an expected value, with standard deviation in brackets. Results show excellent robustness across statistical methodologies.

| Parameter                  | Method | All            |                | Selected       |                |
|----------------------------|--------|----------------|----------------|----------------|----------------|
|                            |        | EB             | HB             | EB             | HB             |
| $\beta_{21}$<br>(NAO)      | MCMC   | 0.140 (0.118)  | 0.140(0.118)   | -              | -              |
|                            | dclone | 0.137(0.053)   | 0.137 (0.053)  | -              | -              |
| $\beta_{22}$<br>(SOI)      | MCMC   | 0.025 (0.061)  | 0.025 (0.061)  | -              | -              |
|                            | dclone | 0.024 (0.027)  | 0.024 (0.027)  | -              | -              |
| $\beta_{23}$<br>(AMO)      | MCMC   | 1.908 (0.434)  | 1.907 (0.435)  | 1.738 (0.385)  | 1.740 (0.386)  |
|                            | dclone | 1.893 (0.193)  | 1.893 (0.194)  | 1.733 (0.172)  | 1.732 (0.173)  |
| $\beta_{24}$<br>Nino-3.4   | MCMC   | -0.223 (0.191) | -0.224 (0.191) | -0.321 (0.147) | -0.321 (0.147) |
|                            | dclone | -0.224 (0.085) | -0.224 (0.085) | -0.321 (0.066) | -0.321 (0.066) |
| $\beta_{25}$<br>(SST)      | MCMC   | 0.033 (0.006)  | 0.033 (0.006)  | 0.031 (0.004)  | 0.031 (0.004)  |
|                            | dclone | 0.034 (0.003)  | 0.034 (0.003)  | 0.031 (0.002)  | 0.031 (0.002)  |
| $\beta_{26}$<br>(Sunspots) | MCMC   | -0.001(0.001)  | -0.001(0.001)  | -              | -              |
|                            | dclone | -0.001(0.001)  | -0.001(0.001)  | -              | -              |
| $\theta_2$                 | MCMC   | 0.390(0.040)   | 0.391(0.040)   | 0.390 (0.040)  | 0.391(0.040)   |
|                            | dclone | 0.389 (0.018)  | 0.390 (0.018)  | 0.389 (0.018)  | 0.390 (0.018)  |
| $\mu_2$                    | MCMC   | 21.121 (0.447) | 21.122(0.436)  | 21.120 (0.448) | 21.121(0.435)  |
|                            | dclone | 21.121 (0.193) | 21.121 (0.192) | 21.121(0.193)  | 21.121 (0.192) |
| $\sigma_2^2$               | MCMC   | 6.997 (1.794)  | 6.644(1.662)   | 6.993(1.798)   | 6.649(1.668)   |
|                            | dclone | 6.508 (0.705)  | 6.445(0.695)   | 6.510(0.705)   | 6.447 (0.695)  |

|                | Estimate | Std. Error | Posterior mean | Posterior SD |
|----------------|----------|------------|----------------|--------------|
| $\alpha_0$     | -0.1919  | 0.0930     | -0.1048        | 0.0842       |
| $\alpha_1$     | -0.2623  | 0.0608     | -0.2723        | 0.0494       |
| $\sigma_{z_1}$ | 1.0395   | 0.0744     | 0.7721         | 0.0302       |
| $\xi_{z_1}$    | -0.5859  | 0.0499     | -0.4335        | 0.0407       |
| $\beta_0$      | 4.3691   | 0.0128     | 4.2243         | 0.0305       |
| $\beta_1$      | 0.3430   | 0.0151     | 0.3508         | 0.0282       |
| $\beta_2$      | -0.0449  | 0.0128     | -0.0434        | 0.0305       |
| $\sigma_{x_1}$ | 0.1429   | 0.0088     | 0.3549         | 0.0169       |
| $\xi_{x_1}$    | -0.3521  | 0.0444     | -0.4875        | 0.0129       |
| $\gamma_0$     | 19.5008  | 0.2033     | 19.2190        | 0.1730       |
| $\gamma_1$     | 0.9391   | 0.5735     | 1.0601         | 0.3632       |
| $\gamma_2$     | 0.5070   | 0.5535     | 0.4400         | 0.3497       |
| $\gamma_3$     | -0.1918  | 0.2068     | -0.1338        | 0.1310       |
| $\sigma_{x_2}$ | 2.2626   | 0.1394     | 1.5064         | 0.0562       |
| $\xi_{x_2}$    | -0.3275  | 0.0373     | -0.1844        | 0.0246       |
| $r$            |          |            | 0.9970         | 0.0039       |

Table 5: Frequentist estimates from models (45), (46), (47), and posterior mean and standard deviation from the trivariate Bayesian extreme value distribution (GEV) model

|               | Post means | Posterior sd | Frequentist est | Freq se |
|---------------|------------|--------------|-----------------|---------|
| $\alpha_0$    | -0.1070    | 0.0859       | -0.1919         | 0.0930  |
| $\alpha_1$    | -0.2720    | 0.0499       | -0.2623         | 0.0608  |
| $\sigma_{z1}$ | 0.7724     | 0.0302       | 1.0395          | 0.0744  |
| $\xi_{z1}$    | -0.4330    | 0.0419       | -0.5859         | 0.0499  |
| $\beta_0$     | 4.2232     | 0.0308       | 4.3691          | 0.0128  |
| $\beta_1$     | 0.3526     | 0.0283       | 0.3430          | 0.0151  |
| $\beta_2$     | -0.0426    | 0.0301       | -0.0449         | 0.0128  |
| $\sigma_{x1}$ | 0.3554     | 0.0171       | 0.1429          | 0.0088  |
| $\xi_{x1}$    | -0.4875    | 0.0128       | -0.3521         | 0.0444  |
| $\gamma_0$    | 20.1867    | 0.1196       | 20.2294         | 0.1831  |
| $\gamma_1$    | 0.8188     | 0.3641       | 0.8162          | 0.5583  |
| $\gamma_2$    | 0.7523     | 0.3531       | 0.7559          | 0.5422  |
| $\gamma_3$    | -0.2522    | 0.1316       | -0.2545         | 0.2012  |
| $\sigma_{x2}$ | 1.4364     | 0.0526       | -               | -       |

Table 6: Frequentist estimates from models (45), (46), (47), and posterior mean and standard deviation from the hierarchical Bayesian model with log-Normal damages

|                                 | minCP      | maxWS       | damages   |
|---------------------------------|------------|-------------|-----------|
| Hierarchical GEV                | 100% (5/5) | 100% (5/5)  | 80% (4/5) |
| Trivariate GEV                  | 100% (5/5) | 100 % (5/5) | 60% (3/5) |
| Hierarchical log-Normal damages | 100% (5/5) | 80% (4/5)   | 60% (3/5) |

Table 7: The proportion of cyclones in 2016-17 where the truth was contained in the 95% credible interval.

| Hurricanes     | minCP  | maxWS  | Damage |
|----------------|--------|--------|--------|
| Hermine (2016) | 0.8440 | 0.5432 | 0.3293 |
| Matthew (2016) | 0.3683 | 0.2023 | 0.1667 |
| Harvey (2017)  | 0.2969 | 0.3514 | 0.0006 |
| Irma (2017)    | 0.1964 | 0.1638 | 0.0430 |
| Nate (2017)    | 0.9263 | 0.0516 | 0.4689 |

Table 8: For the hierarchical GEV model in Section C.1,  $\delta$  values for each of the hurricanes, closer to 1 reflects the truth to be close to the median of the posterior predictive distribution and closer to 0 reflects the truth lying in the tails of the distribution.



| Hurricanes     | minCP  | maxWS  | Damage |
|----------------|--------|--------|--------|
| Hermine (2016) | 0.8256 | 0.5392 | 0.3424 |
| Matthew (2016) | 0.3823 | 0.2019 | 0.2104 |
| Harvey (2017)  | 0.3038 | 0.3525 | 2e-04  |
| Irma (2017)    | 0.2009 | 0.1656 | 0.0355 |
| Nate (2017)    | 0.9159 | 0.0491 | 0.4783 |

Table 9: For the hierarchical GEV model with log-Normal damages in Section C.2,  $\delta$  values for each of the hurricanes, closer to 1 reflects the truth to be close to the median of the posterior predictive distribution and closer to 0 reflects the truth lying in the tails of the distribution.

## E Appendix:All Figures

Figure 5: Posterior predictive distributions for 2016 low intensity cyclones. The top row is for empirical Bayes prediction, the middle row is for fast Bayesian prediction and the bottom row is for hierarchical Bayesian prediction. The left column is the probability mass function for cyclone frequency, middle column is for damage-inflicting probability, and right column is density for logarithm of damages. The actual values are displayed with red dashed lines.

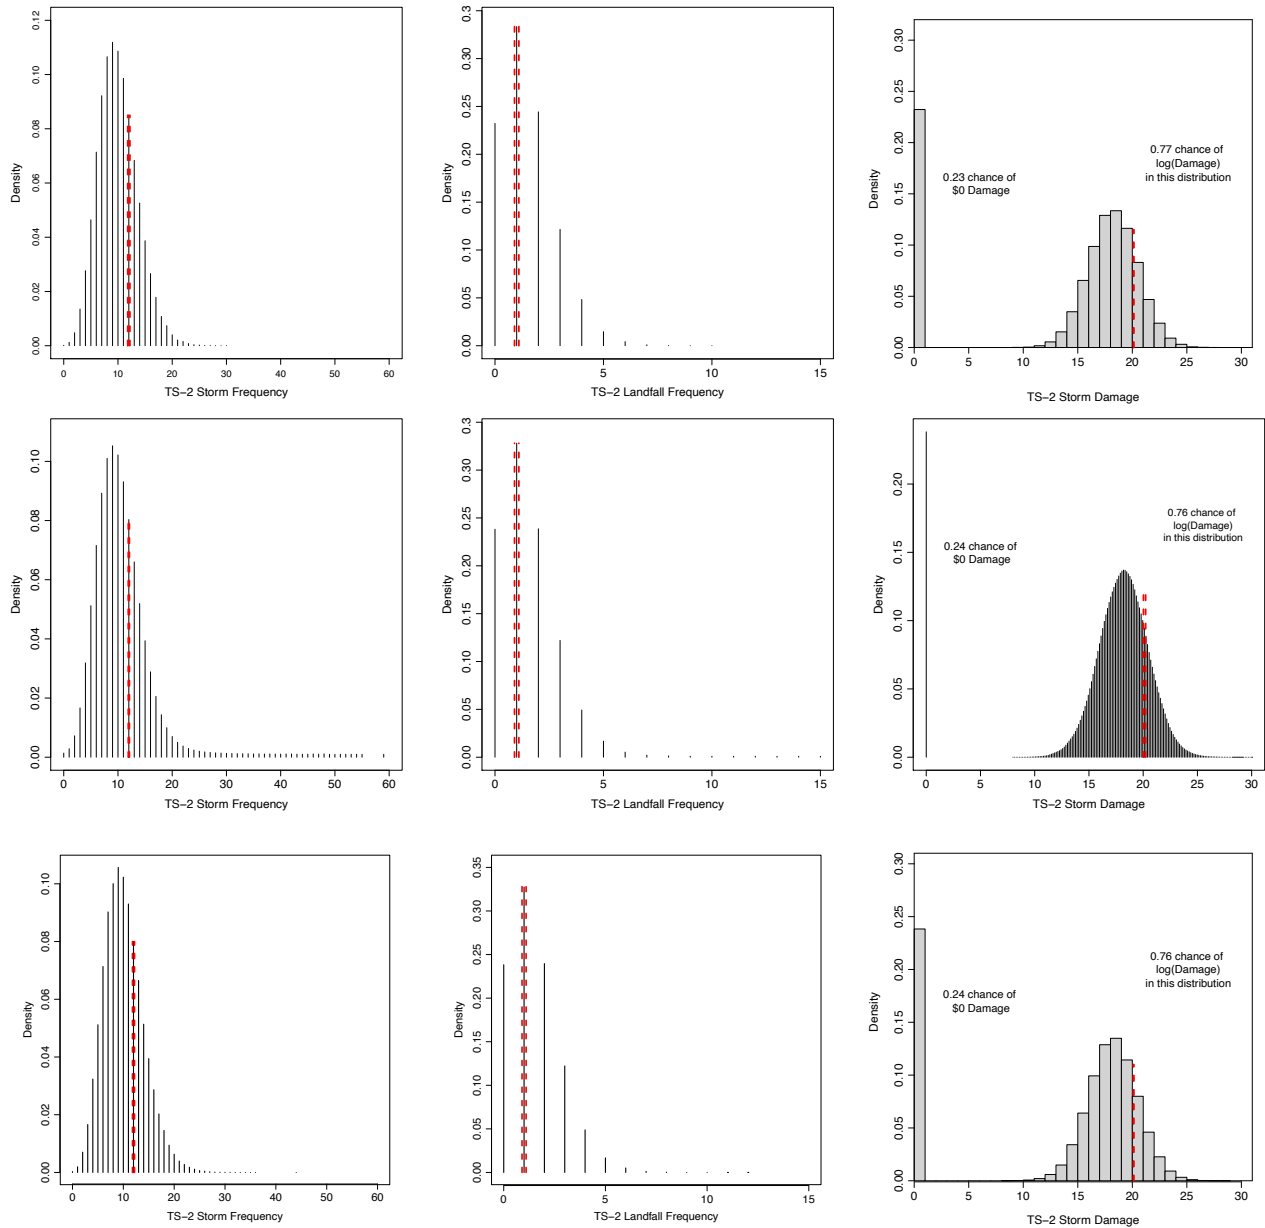

Figure 6: Posterior Predictive Distributions for 2016 High Intensity cyclones. The top row is for empirical Bayes prediction, the middle row is for fast Bayesian prediction and the bottom row is for hierarchical Bayesian prediction. The left column is the probability mass function for cyclone frequency, middle column is for damage-inflicting probability, and right column is density for logarithm of damages. The actual values are displayed with red dashed lines.

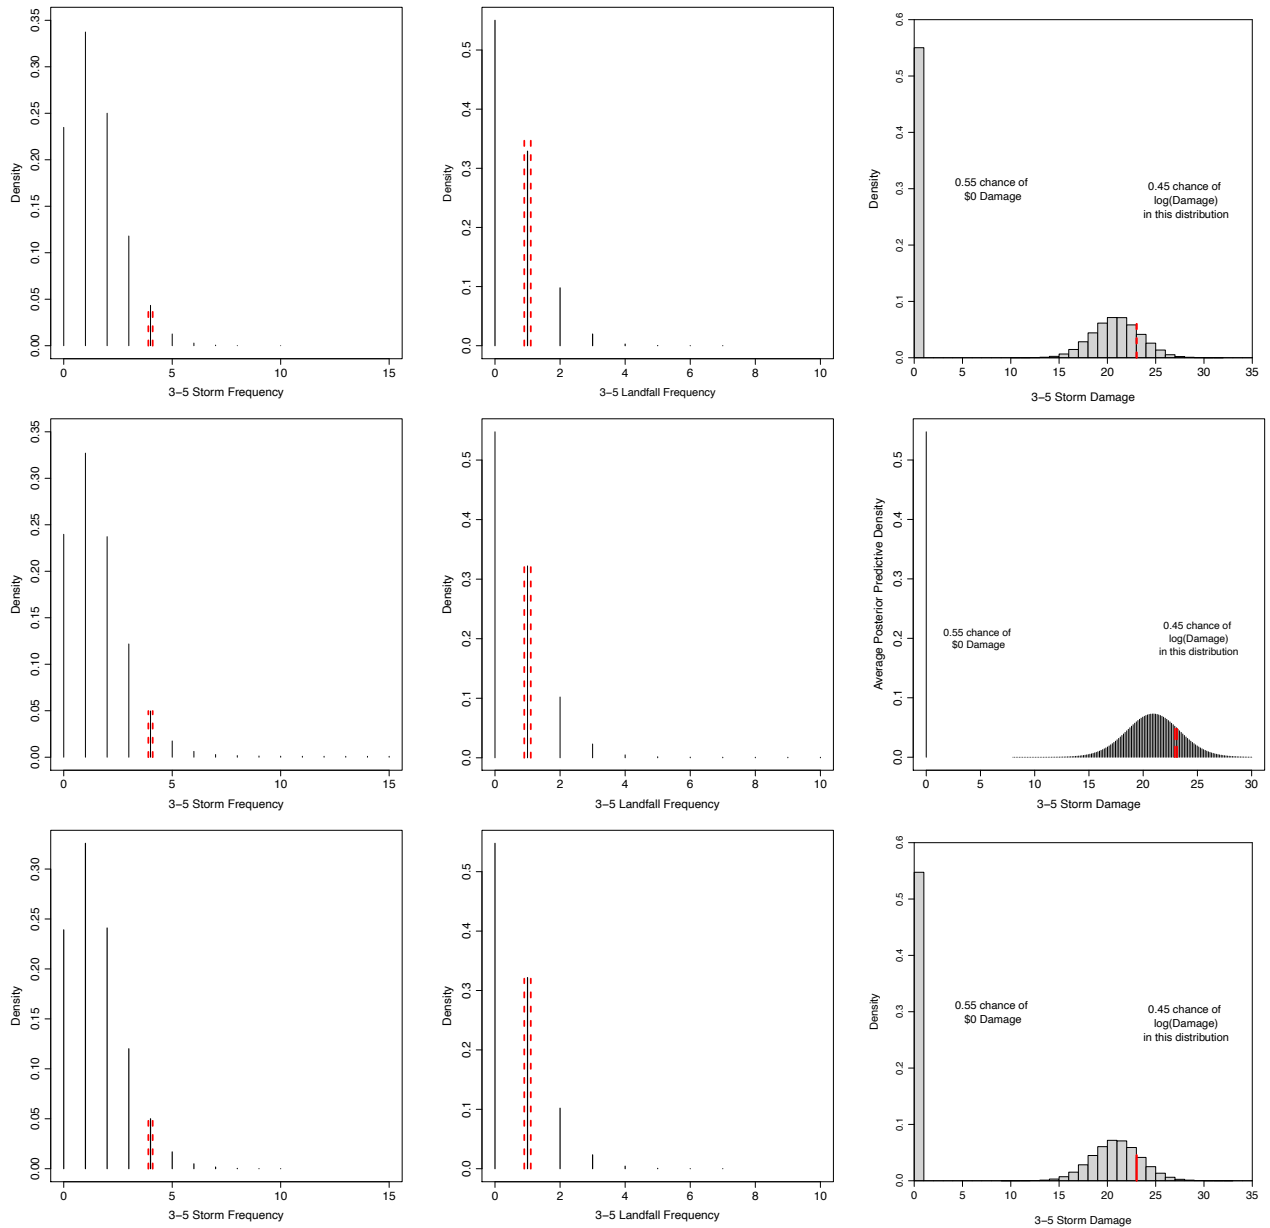

Figure 7: Posterior Predictive Distributions for 2017 Low Intensity cyclones. The top row is for empirical Bayes prediction, the middle row is for fast Bayesian prediction and the bottom row is for hierarchical Bayesian prediction. The left column is the probability mass function for cyclone frequency, middle column is for damage-inflicting probability, and right column is density for logarithm of damages. The actual values are displayed with red dashed lines.

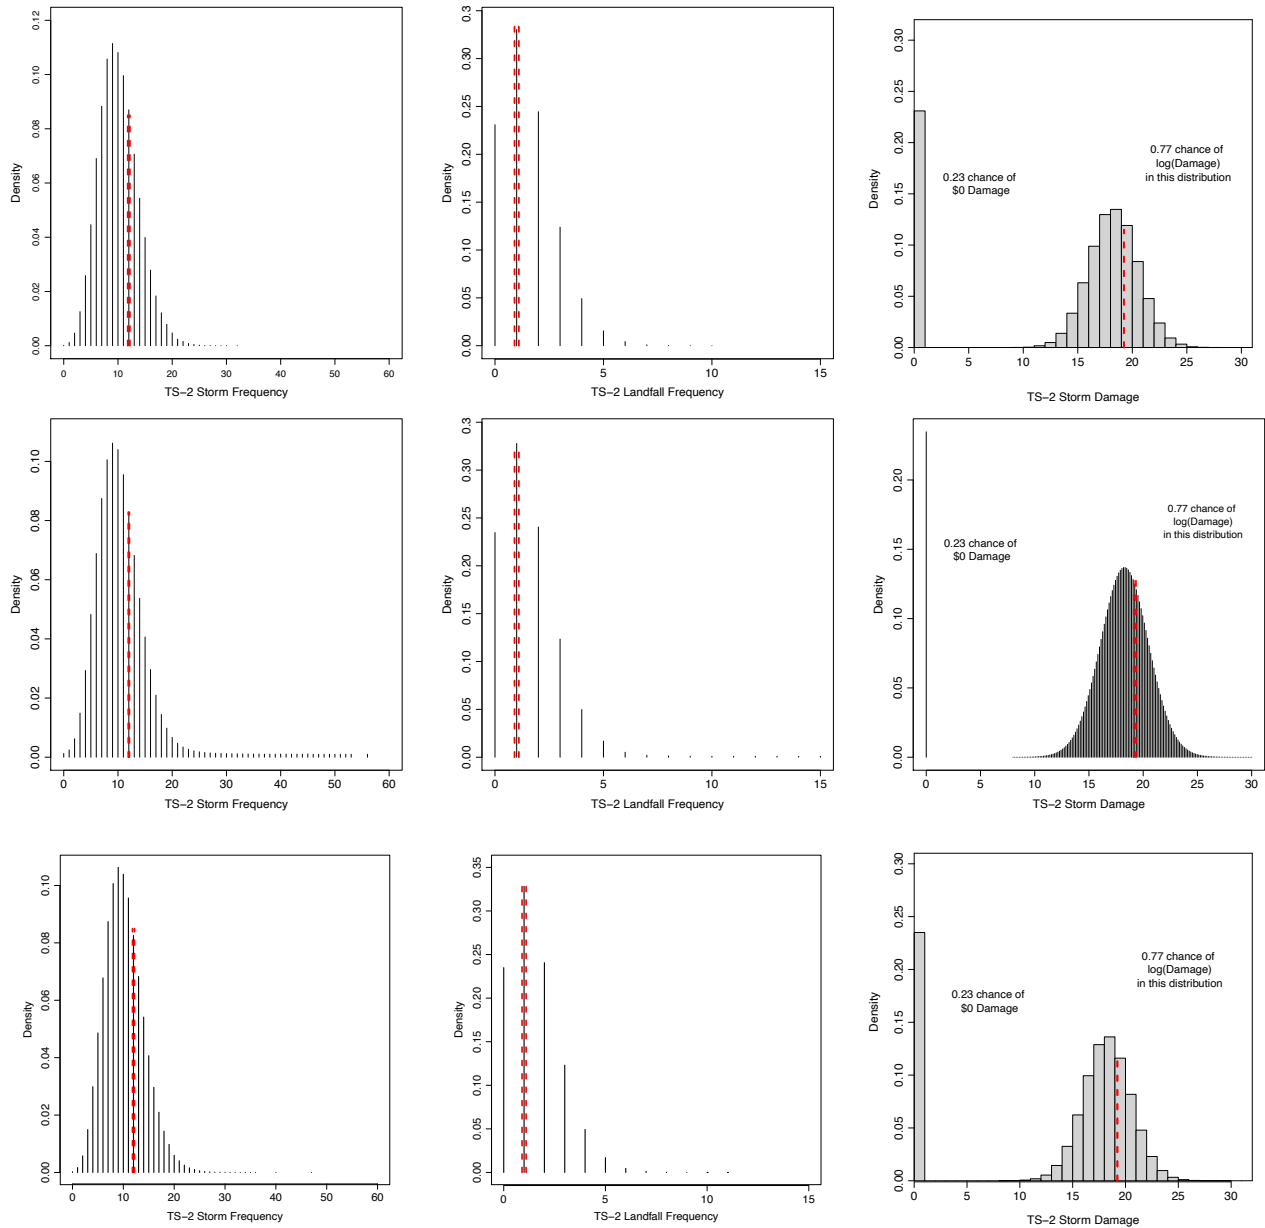

Figure 8: Posterior Predictive Distributions for 2017 High Intensity cyclones. The top row is for empirical Bayes prediction, the middle row is for fast Bayesian prediction and the bottom row is for hierarchical Bayesian prediction. The left column is the probability mass function for cyclone frequency, middle column is for damage-inflicting probability, and right column is density for logarithm of damages. The actual values are displayed with red dashed lines.

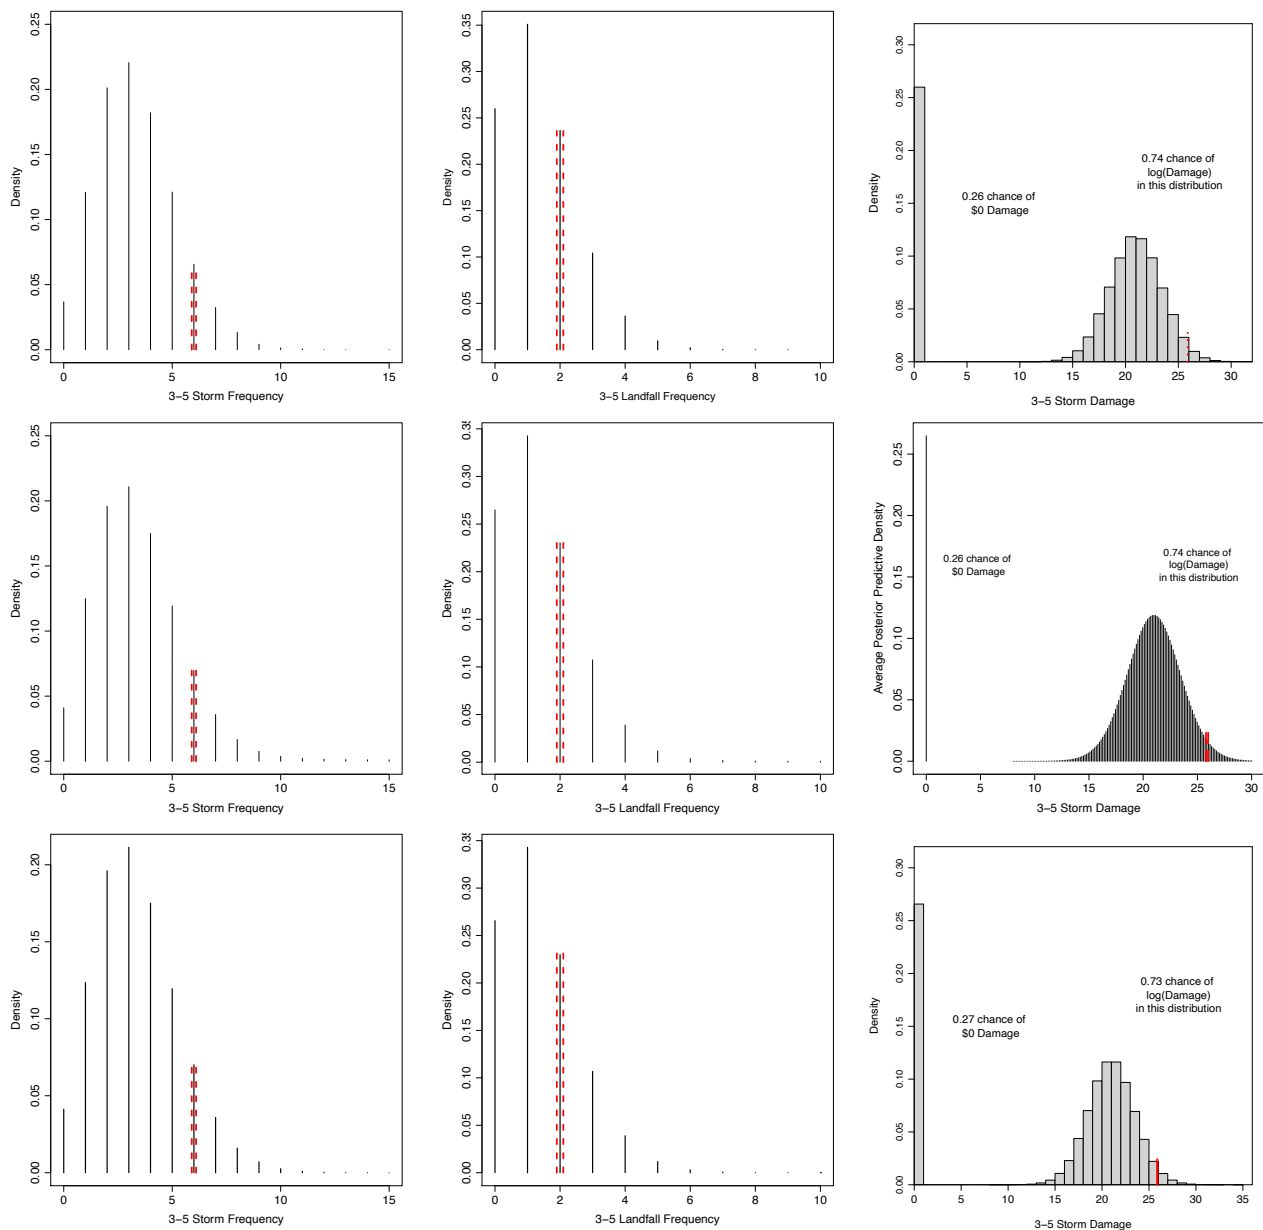

Figure 9: Posterior Predictive Distributions for 2018 Low Intensity cyclones. The top row is for empirical Bayes prediction, the middle row is for fast Bayesian prediction and the bottom row is for hierarchical Bayesian prediction. The left column is the probability mass function for cyclone frequency, middle column is for damage-inflicting probability, and right column is density for logarithm of damages. The actual values are displayed with red dashed lines.

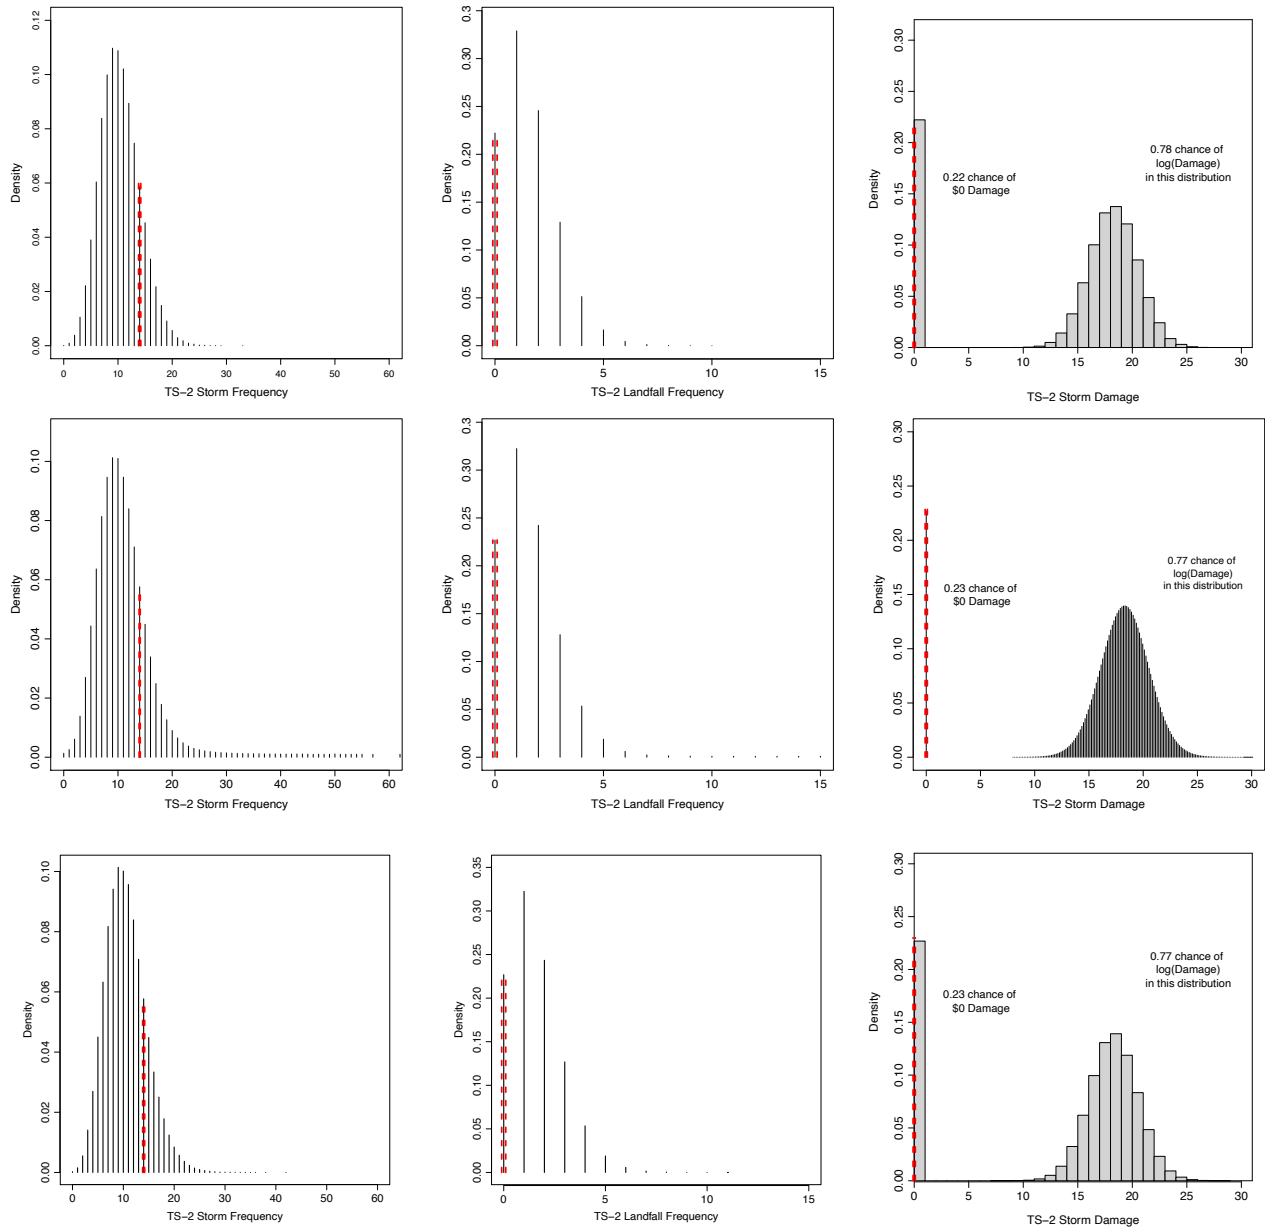

Figure 10: Posterior Predictive Distributions for 2018 High Intensity cyclones. The top row is for empirical Bayes prediction, the middle row is for fast Bayesian prediction and the bottom row is for hierarchical Bayesian prediction. The left column is the probability mass function for cyclone frequency, middle column is for damage-inflicting probability, and right column is density for logarithm of damages. The actual values are displayed with red dashed lines.

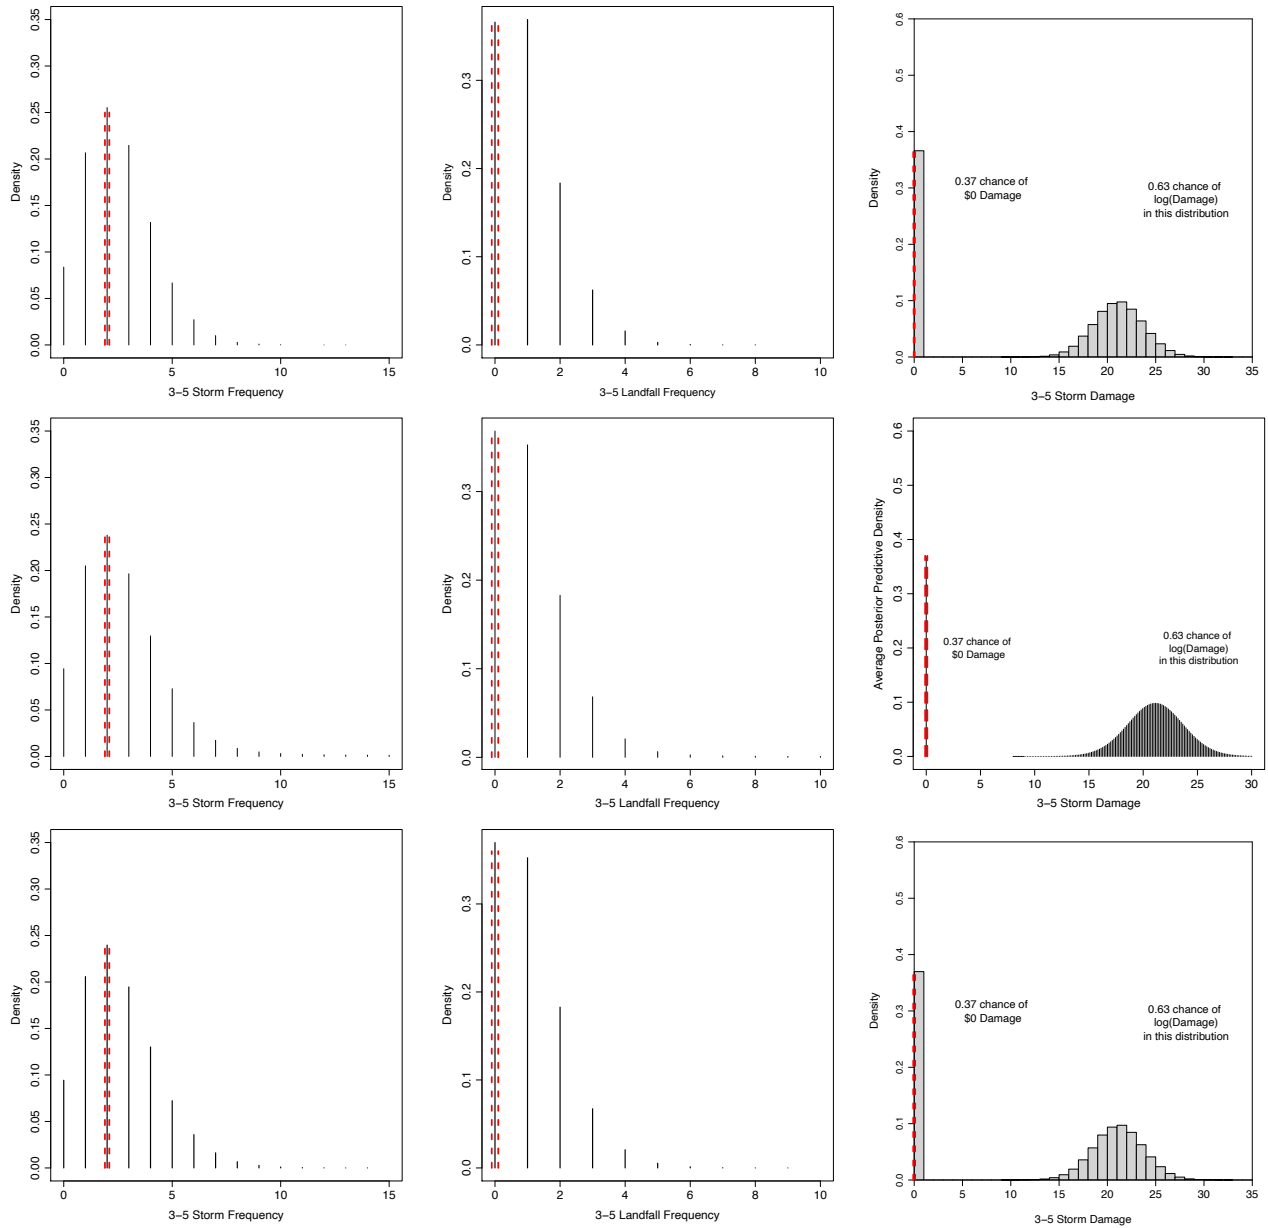



Figure 11: Posterior Predictive Distributions for 2019 Low Intensity cyclones. The top row is for empirical Bayes prediction, the middle row is for fast Bayesian prediction and the bottom row is for hierarchical Bayesian prediction. The left column is the probability mass function for cyclone frequency, middle column is for damage-inflicting probability, and right column is density for logarithm of damages. The actual values are displayed with red dashed lines.

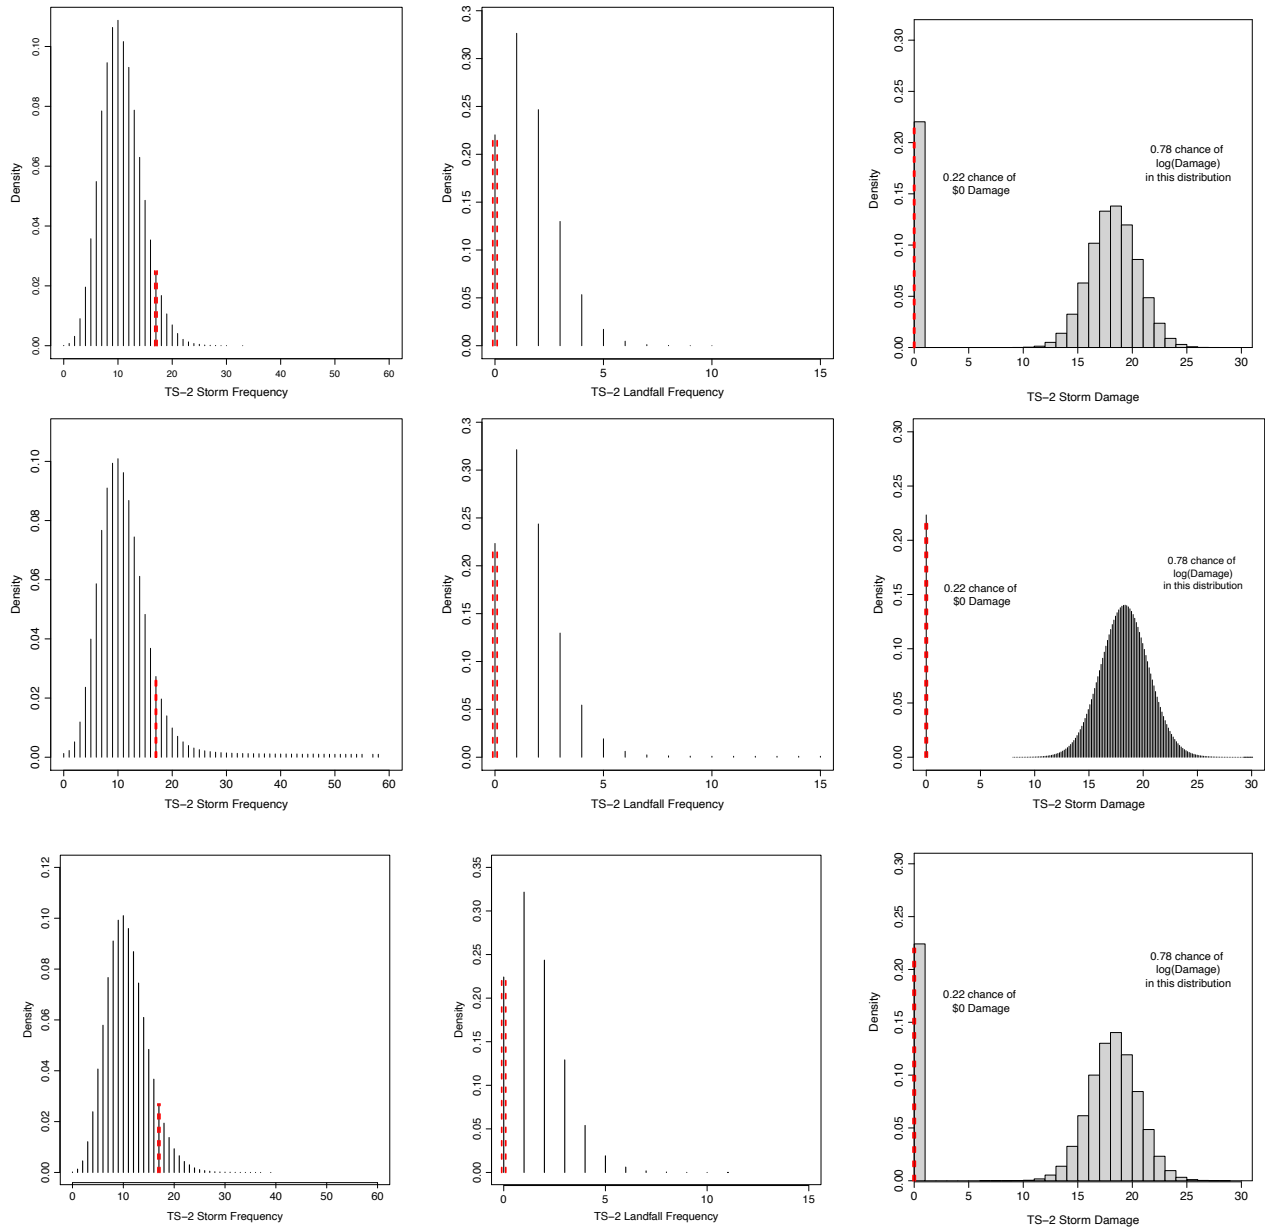

Figure 12: Posterior Predictive Distributions for 2019 High Intensity cyclones. The top row is for empirical Bayes prediction, the middle row is for fast Bayesian prediction and the bottom row is for hierarchical Bayesian prediction. The left column is the probability mass function for cyclone frequency, middle column is for damage-inflicting probability, and right column is density for logarithm of damages. The actual values are displayed with red dashed lines.

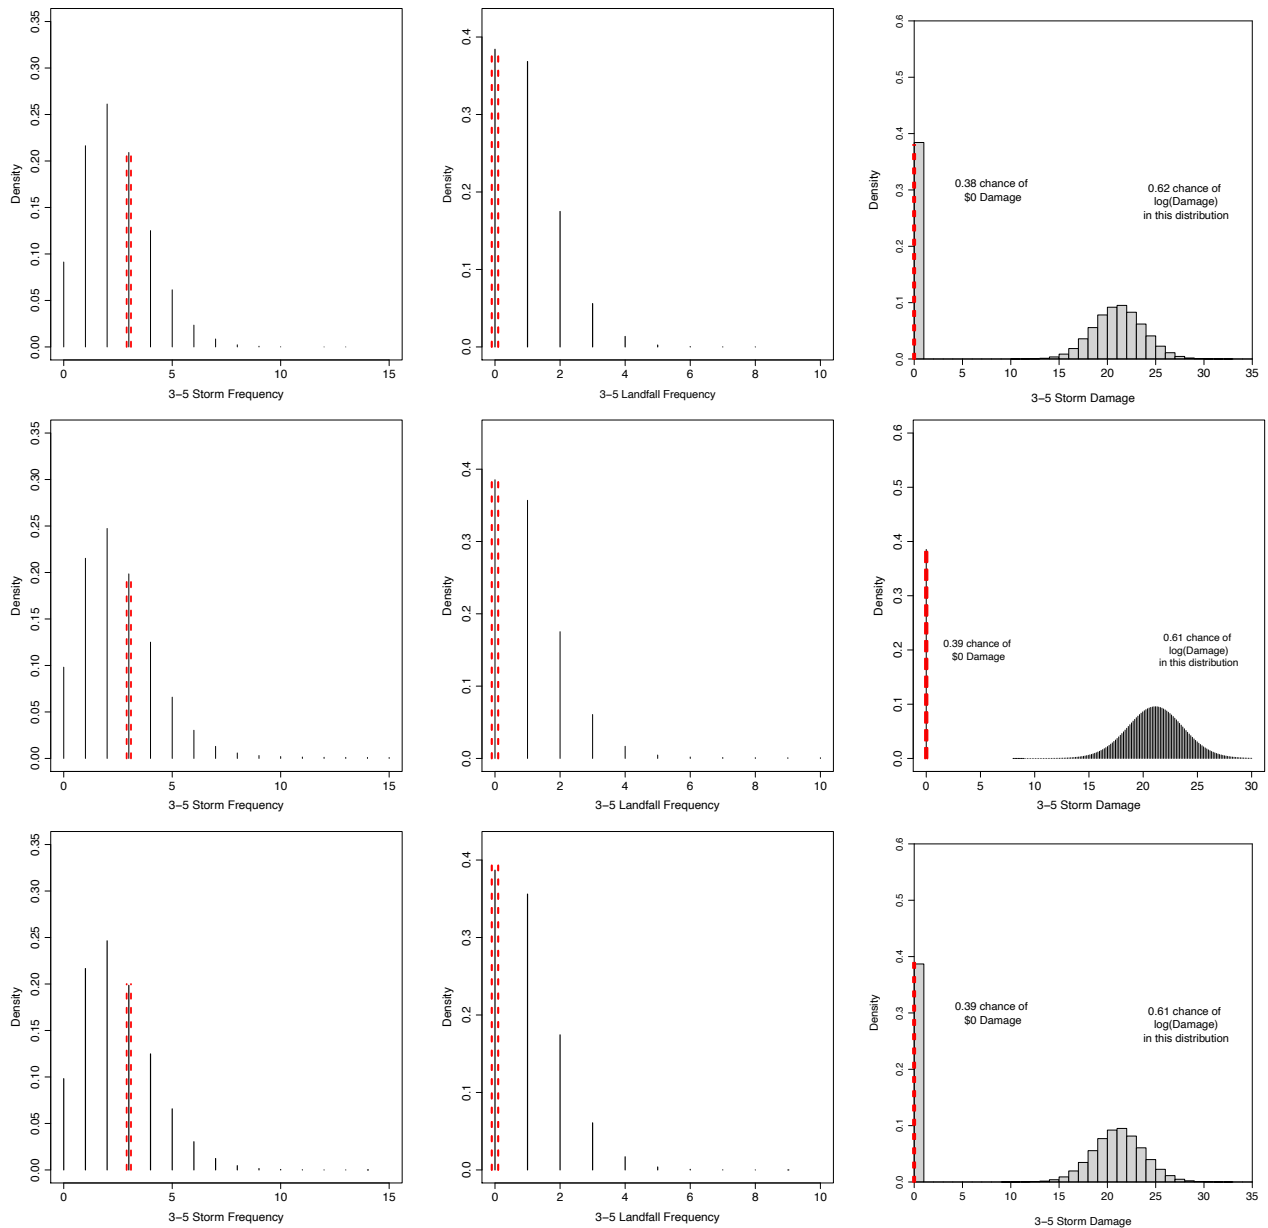

Supplement: Supplementary file 1 [file BayesianStorm_Supple_08_16_2022.pdf]
